# Supplementary material for: No Corners Cut: State-Grounded Transitions for Mid-Stream Prompt Switches in Video Generation
Source: arXiv:2609.38691 source file (2026-11-18)
Supplement: Supplementary file 2 [file statements.tex]

\section{Author Statements}
\subsection*{AI use statement}

In this work, we used generative AI tools to assist with dataset construction and filtering, including the generation and verification of candidate training and benchmark data. Generative models are also used as explicit components of our approach pipeline, including LLM/VLM-based data processing and the VLM planner used during inference; these components and their roles are described in the corresponding method and experimental sections.

Additionally, generative AI tools were used to assist with experimental code development and debugging, and language editing and polishing of author-written manuscript drafts.

All AI-assisted data construction and filtering were subject to programmatic checks and human inspection. AI-assisted code was reviewed and tested by the authors, and all AI-assisted manuscript edits were reviewed by the authors. We take responsibility for the final content of this work, including text, claims, code, data, and artifacts produced with the aid of generative AI.

\subsection*{Ethics statement}

This work builds on the publicly available Wan2.1-T2V models.
We introduce \bench{}, whose prompts are generated from structured specifications
with LLM assistance and subsequently inspected by the authors.
The benchmark contains no personal or private data.
Some cases refer to fictional characters solely for evaluating identity preservation;
these names are used only as textual generation conditions and are not associated
with real individuals.

We plan to release the \bench{} prompts, annotations, and metadata under the
Creative Commons Attribution 4.0 International (CC BY 4.0) license, and the
evaluation code under the Apache License 2.0.
The final release terms will be subject to institutional legal review and
compatibility with the licenses of upstream models and resources.

For the user study (Sec.~\ref{app:user-study}) and the
human-alignment study (Sec.~\ref{app:human-alignment}),
we recruited two disjoint groups of 12 participants each.
The human-alignment participants were fellow students.
In both studies, participants compared anonymized generated
clips with method identities hidden. Participants were informed
of the study procedures before participation and provided
informed consent. Neither study collected sensitive personal
information. Neither study was subject to formal ethics
review under our institutional policy.

As with other video-generation systems, improved controllability may be misused
to create misleading or deceptive visual content.
We encourage responsible use of the released benchmark, models, and evaluation tools.

\subsection*{Reproducibility statement}

Sec.~3 (Method) of the main paper specifies the planner and \cdmd{}, and Sec.~5 (Experiments) of the main paper lists the backbone, sampler, and training hyperparameters. Sec.~\ref{app:agent_inference} gives the planner inputs and prompts, Sec.~\ref{app:benchmark} the benchmark construction, evaluator, and temporal sampling, Sec.~\ref{app:checklists} all checklist criteria, and Sec.~\ref{app:training_data_construction} the construction of the training schedules.
Detailed training settings are provided in Sec.~\ref{app:training_hyperparameters}.
